# Supplementary material for: FusionRCG: Orchestrating Recursive Computation Graphs across GPU Memory Hierarchies
Source: arXiv:2605.10312 source file (2026-05-13)
Supplement: Supplementary file 1 [file appendix.tex]

% =====================================================================
% APPENDIX: Detailed Experimental Tables
% =====================================================================
\appendix

\section{Detailed Experimental Tables}
\label{sec:appendix-tables}

% ── Table A: DSA Scheduling Ablation ─────────────────────────────────
\begin{table}[h]
\caption{DSA scheduling ablation. Spill is \texttt{ptxas}-reported total (store$+$load); local sectors are Nsight Compute dynamic load$+$store.}
\begin{center}
\small
\begin{tabular}{llrrr}
\toprule
Quartet & Variant & Throughput & Spill (B) & Local sec. \\
\midrule
\multirow{2}{*}{$(0,0,0,0)$} & Full & 32.65M & 0 & 0 \\
 & No DSA & 33.37M & 0 & 0 \\
\midrule
\multirow{2}{*}{$(1,1,1,1)$} & Full & 16.37M & 776 & 7{,}168 \\
 & No DSA & 16.35M & 960 & 8{,}128 \\
\midrule
\multirow{2}{*}{$(2,1,2,1)$} & Full & 5.86M & 28{,}312 & 164{,}416 \\
 & No DSA & 5.69M & 29{,}696 & 176{,}096 \\
\midrule
\multirow{2}{*}{$(2,2,2,2)$} & Full & 1.33M & 768 & 13{,}248 \\
 & No DSA & 1.12M & 54{,}216 & 440{,}576 \\
\midrule
\multirow{2}{*}{$(3,2,2,1)$} & Full & 1.40M & 408 & 7{,}680 \\
 & No DSA & 1.30M & 41{,}648 & 337{,}024 \\
\midrule
\multirow{2}{*}{$(4,2,2,1)$} & Full & 1.05M & 1{,}040 & 12{,}736 \\
 & No DSA & 0.88M & 74{,}992 & 604{,}928 \\
\bottomrule
\end{tabular}
\label{tab:dsa}
\end{center}
\end{table}

% ── Table B: Spherical Fusion Ablation ───────────────────────────────
\begin{table}[h]
\caption{Spherical fusion ablation. $n_\mathrm{cart}$/$n_\mathrm{sph}$: four-index tensor element counts in Cartesian/spherical basis. Theory: $n_\mathrm{cart}/n_\mathrm{sph}$. DRAM and L1/TEX ratios: No-spherical\,/\,Full (${>}1$ means the Cartesian variant moves more data).}
\begin{center}
\small
\begin{tabular}{lrrrrrr}
\toprule
Quartet & $n_\mathrm{c}$ & $n_\mathrm{s}$ & Theory & Gain & \shortstack{DRAM\\ratio} & \shortstack{L1/TEX\\ratio} \\
\midrule
$(0,0,0,0)$ & 1 & 1 & 1.00$\times$ & 0.97$\times$ & 1.01 & 1.00 \\
$(1,1,0,0)$ & 9 & 9 & 1.00$\times$ & 1.00$\times$ & 1.01 & 1.00 \\
$(2,1,1,1)$ & 162 & 135 & 1.20$\times$ & 1.06$\times$ & 1.11 & 1.25 \\
$(3,2,2,1)$ & 1{,}080 & 525 & 2.06$\times$ & 1.38$\times$ & 0.98 & 1.29 \\
$(4,3,3,2)$ & 9{,}000 & 2{,}205 & $\mathbf{4.08\times}$ & $\mathbf{2.99\times}$ & $\mathbf{8.49}$ & 1.36 \\
\bottomrule
\end{tabular}
\label{tab:spherical}
\end{center}
\end{table}

% ── Table C: Adaptive Multi-Tier Routing ─────────────────────────────
\begin{table*}[h]
\caption{Adaptive multi-tier routing across the angular-momentum ladder ($\sum l_i = 0$--$16$). ``Full'' uses adaptive Tier~1/Tier~2 routing; ``T1 only'' forces Tier~1. Dashes indicate pathological timing or compilation failure. Spill is \texttt{ptxas}-reported total (store$+$load).}
\begin{center}
\small
\begin{tabular}{rllrrrrrrl}
\toprule
$\sum l$ & Quartet & Tier & Full (q/s) & T1 only (q/s) & Ratio & Full spill & T1 spill & Full local sec. & Status \\
\midrule
0 & $(0,0,0,0)$ & T1 & 33.8M & 32.7M & 1.03$\times$ & 0\,B & 0\,B & 0 & identical \\
1 & $(1,0,0,0)$ & T1 & 29.9M & 30.3M & 0.99$\times$ & 0\,B & 0\,B & 384 & identical \\
2 & $(1,1,0,0)$ & T1 & 26.9M & 27.5M & 0.98$\times$ & 0\,B & 0\,B & 576 & identical \\
3 & $(1,1,1,0)$ & T1 & 23.0M & 22.8M & 1.01$\times$ & 0\,B & 0\,B & 768 & identical \\
4 & $(1,1,1,1)$ & T1 & 16.1M & 16.2M & 0.99$\times$ & 776\,B & 776\,B & 7.2K & identical \\
5 & $(2,1,1,1)$ & T1 & 10.7M & 10.6M & 1.01$\times$ & 9.2\,KB & 9.2\,KB & 58.8K & identical \\
6 & $(2,2,1,1)$ & T1 & 5.78M & 5.77M & 1.00$\times$ & 27.7\,KB & 27.7\,KB & 164K & identical \\
\midrule
7 & $(2,2,2,1)$ & T2 & 2.04M & 2.85M & 0.72$\times$ & 144\,B & 58.9\,KB & 3.6K & crossover \\
\midrule
8 & $(2,2,2,2)$ & T2 & 1.33M & 1.09M & 1.22$\times$ & 768\,B & 165\,KB & 13.2K & adaptive wins \\
9 & $(3,2,2,2)$ & T2 & 935K & 714K & 1.31$\times$ & 1.4\,KB & 259\,KB & 18.2K & adaptive wins \\
10 & $(3,3,2,2)$ & T2 & 612K & --- & --- & 5.9\,KB & 486\,KB & 56.2K & T1 pathological \\
11 & $(3,3,3,2)$ & T2 & 423K & --- & --- & 23.6\,KB & 764\,KB & 204K & T1 pathological \\
12 & $(3,3,3,3)$ & T2 & 234K & --- & --- & 49.3\,KB & 1.30\,MB & 429K & T1 pathological \\
13 & $(4,3,3,3)$ & T2 & 145K & --- & --- & 91.3\,KB & --- & 948K & T1 compile fail \\
14 & $(4,4,3,3)$ & T2 & 785K & --- & --- & 10.5\,KB & --- & 86.3K & MD route \\
15 & $(4,4,4,3)$ & T2 & 654K & --- & --- & 16.0\,KB & --- & 132K & MD route \\
16 & $(4,4,4,4)$ & T2 & 441K & --- & --- & 23.8\,KB & --- & 200K & MD route \\
\bottomrule
\end{tabular}
\label{tab:multitier}
\end{center}
\end{table*}

% ── Table D: Component Summary ───────────────────────────────────────
\begin{table}[h]
\caption{Representative measurements tying each method component to an observable hardware effect.}
\begin{center}
\scriptsize
\begin{tabular}{p{0.13\columnwidth}p{0.14\columnwidth}p{0.63\columnwidth}}
\toprule
Component & Case & Evidence \\
\midrule
Axis priority & \shortstack[l]{$(1,1,1,1)$\\$(4,3,3,2)$} & Offline $\mathrm{PeakLive}$ reduced by 42\% on $(1,1,1,1)$. On $(4,3,3,2)$: 82.6K\,q/s vs.\ 73.1K with axis off ($+$12.9\%). \\
\addlinespace
DSA & $(2,2,2,2)$ & $1.19\times$ throughput (1.33M vs.\ 1.12M\,q/s). Spill $70.6\times$ lower; local sectors $33.3\times$ lower. \\
\addlinespace
Spherical & $(4,3,3,2)$ & $2.99\times$ throughput (289K vs.\ 96.7K\,q/s). DRAM $8.49\times$ lower; L1/TEX $1.36\times$ lower. \\
\addlinespace
Tiering & $(3,2,2,2)$ & $1.31\times$ throughput (935K vs.\ 714K\,q/s). Local sectors $94.8\times$ lower; DRAM $2.83\times$ lower. On sum-$l$ ladder: T1 for 7, T2 for 10 quartets. \\
\bottomrule
\end{tabular}
\label{tab:method-summary}
\end{center}
\end{table}

% ── Table E: Multi-Stream Scaling ────────────────────────────────────
\begin{table}[h]
\caption{Multi-stream scaling. Effective throughput measures aggregate kernel processing rate across all concurrent streams.}
\begin{center}
\small
\begin{tabular}{llrrrr}
\toprule
Quartet & $\sum l$ & Streams & \shortstack{Total\\(ms)} & \shortstack{Eff.\\(lnch/ms)} & \shortstack{Scale\\vs.\ 1} \\
\midrule
\multirow{3}{*}{$(2,2,2,2)$} & \multirow{3}{*}{8} & 1 & 2.36 & 4.24 & 1.00$\times$ \\
 & & 2 & 2.50 & 8.01 & 1.89$\times$ \\
 & & 4 & 2.75 & 14.56 & 3.44$\times$ \\
\midrule
\multirow{3}{*}{$(3,3,3,3)$} & \multirow{3}{*}{12} & 1 & 13.28 & 0.75 & 1.00$\times$ \\
 & & 2 & 17.25 & 1.16 & 1.54$\times$ \\
 & & 4 & 20.93 & 1.91 & 2.54$\times$ \\
\midrule
\multirow{3}{*}{$(4,4,4,3)$} & \multirow{3}{*}{15} & 1 & 4.58 & 2.18 & 1.00$\times$ \\
 & & 2 & 6.69 & 2.99 & 1.37$\times$ \\
 & & 4 & 11.18 & 3.58 & 1.64$\times$ \\
\bottomrule
\end{tabular}
\label{tab:multistream}
\end{center}
\end{table}
